# Supplementary material for: AuroraCap: Efficient, Performant Video Detailed Captioning and a New Benchmark
Source: arXiv:2410.03051 source file (2025-04-09)
Supplement: Supplementary file 1 [file 1_training_datasets.tex]

\section{Training Datasets}
\label{sec:training_datasets}

\paragraph{LAION-CC-SBU-595K~\cite{liu2024visual}~(595K)} Filtered from LAION~\cite{schuhmann2022laion}, CC3M~\cite{changpinyo2021conceptual}, and SBU~\cite{ordonez2011im2text} dataset based on the number of noun-phrases words preprocessed by LLaVA~\cite{liu2024visual}. 

\paragraph{ShareGPT4V-PT~\cite{chen2023sharegpt4v}~(1,246K)} A pioneering large-scale resource featuring 1.2 million highly descriptive captions, which surpasses existing datasets in diversity and information content, covering world knowledge, object properties, spatial relationships, and aesthetic
evaluations generated by Share-Captioner~\cite{chen2023sharegpt4v}. 

\paragraph{Image-Paragraph-Captioning~\cite{krause2017hierarchical}~(14K)} All the images are part of the Visual Genome dataset~\cite{krishna2017visual}, each image also contains 50 region descriptions (short phrases describing parts of an image), 35 objects, 26 attributes and 21 relationships and 17 question-answer pairs.

\paragraph{MS COCO~\cite{lin2014microsoft}~(567K)} The COCO Caption dataset contains diverse images with over one and a half million detailed captions, widely used for image captioning and image-text retrieval tasks.

\paragraph{TextCaps~\cite{sidorov2020textcaps}~(98K)} TextCaps tasks a model with identifying text, contextualizing it within its visual surroundings, and determining which portion of the text to replicate or rephrase. Optical Character Recognition (OCR) tokens are employed in the training process.

\paragraph{COST~\cite{jain2023vcoder}~(100K)} Incorporate the images from COCO~\cite{lin2014microsoft}, the questions from GPT-4, and the segmentation outputs from OneFormer~\cite{jain2023oneformer} in a question-answer format for training and evaluating MLLMs on the object identification task. COST also support the object order perception task by incorporating depth map outputs from DINOv2~\cite{oquab2023dinov2} pretrained DPT~\cite{ranftl2021vision}.

\paragraph{ChatterBox~\cite{tian2024chatterbox}~(76K)} Spans challenges including multi-round dialogue, complex spatial relationships among
multiple instances, and consistent reasoning. We only use the Multi-round Referring and Grounding (CB-MRG) subset, which using GPT-4 to generate questions and answers that focus on instance-level relationship. Provided with related instances, GPT-4 shall write dialogues using their relationship.

\paragraph{V*~\cite{wu2023textit}~(262K)} This data consists of four parts: GQA
data (70k)~\cite{hudson2019gqa}, VQA data focused on object attributes (51k) from VAW~\cite{pham2021learning}, VQA data focused on spatial relationship (46k), and 100K negative data for target objects reasoning about 1) if required to answer the question, and 2) if missing or not clear enough in image.

\paragraph{COCO-GOI~\cite{lin2014microsoft}~(30K)} The COCO-GOI dataset adds an extra layer of information by annotating interactions between objects in these images.

\paragraph{COCO-Text~\cite{veit2016coco}~(118K)} Each image is annotated with bounding boxes around text regions, as well as transcription of the text.

\paragraph{ImageNet~\cite{russakovsky2015imagenet}~(30K)} ImageNet is a large-scale visual database designed for use in visual object recognition research, consisting of over 1 million images across 1K different classes.

\paragraph{COCO-ITM~\cite{lin2014microsoft}~(30K)} The COCO-ITM (Image-Text Matching) dataset is an extension of the COCO (Common Objects in Context) dataset, specifically designed for tasks involving the relationship between images and text. 

\paragraph{e-SNLI-VE~\cite{kayser2021vil}~(20K)} The e-SNLI-VE (Extended SNLI-Visual Entailment) dataset is a multimodal dataset designed for visual entailment tasks. It extends the Stanford Natural Language Inference (SNLI) corpus to include visual information for visual entailment research.

\paragraph{Mocheg~\cite{yao2023end}~(5K)} MOCHEG (Multi-Object and Contextual Hierarchical Graphs) is a dataset or framework designed to facilitate research in visual relationship detection and scene understanding. 

\paragraph{IQA~\cite{duanmu2021quantifying}~(5K)} Image quality assessment (IQA) dataset aim to establish a quantitative relationship between visual images and their quality as perceived by human observers.

\paragraph{CLEVR~\cite{johnson2017clevr}~(30K)} CLEVR (Compositional Language and Elementary Visual Reasoning) is a diagnostic dataset designed to test the visual reasoning capabilities of AI models. It was created to address the limitations of previous visual question answering (VQA) datasets, which often include biases that models can exploit without truly understanding the visual content.

\paragraph{NLVR~\cite{suhr2017corpus}~(29K)} NLVR (Natural Language for Visual Reasoning) is a dataset and benchmark designed to evaluate the ability of AI models to perform reasoning tasks involving natural language and visual inputs. It was created to advance the field of visual reasoning and to test the models' ability to understand and reason about natural language descriptions of complex scenes.

\paragraph{VCR~\cite{zellers2019recognition}~(25K)} VCR (Visual Commonsense Reasoning) is a dataset designed to push the boundaries of visual understanding and reasoning in AI models. It goes beyond traditional visual question answering by requiring models to understand and reason about scenes at a deeper level, incorporating commonsense knowledge and inferencing abilities.

\paragraph{VisualMRC~\cite{tanaka2021visualmrc}~(15K)} VisualMRC (Visual Machine Reading Comprehension) is a dataset and benchmark designed to evaluate the ability of comprehend visual information in conjunction with textual information. It aims to push the boundaries of multimodal understanding, requiring models to integrate and reason about both visual and textual inputs to answer questions

\paragraph{Winoground~\cite{thrush2022winoground}~(1K)} Winoground is a dataset designed to evaluate the capability of models to understand and reason about multimodal ambiguities and challenges in visual and linguistic contexts. It is inspired by the Winograd Schema Challenge, which is used to test common-sense reasoning in natural language processing, but extends this challenge to include visual information.

\paragraph{VQA v2~\cite{goyal2017making}~(30K)} VQAv2 (Visual Question Answering v2) is a widely used dataset in the field of computer vision and natural language processing, designed to advance research in visual question answering (VQA). This dataset addresses some of the limitations of the original VQA dataset by providing more balanced and challenging questions. 

\paragraph{Shapes VQA~\cite{andreas2016neural}~(14K)} Shapes VQA is a synthetic dataset designed to evaluate the visual reasoning capabilities of models in a controlled environment. This dataset focuses on simple geometric shapes and their attributes, allowing researchers to study the fundamental aspects of visual question answering without the complexities and biases of natural images. 

\paragraph{DocVQA~\cite{mathew2021docvqa}~(40K)} DocVQA (Document Visual Question Answering) is a dataset and benchmark specifically designed to evaluate the ability of models to understand and answer questions about document images. This dataset focuses on visual question answering in the context of various types of documents, such as forms, invoices, reports, and more.

\paragraph{OK-VQA~\cite{marino2019ok}~(9K)} OK-VQA (Open-Ended Knowledge Visual Question Answering) is a dataset designed to evaluate the ability of models to answer questions about images using external knowledge beyond what is explicitly shown in the image. This dataset challenges models to integrate visual understanding with world knowledge and common sense reasoning. 

\paragraph{GQA~\cite{hudson2019gqa}~(30K)} The GQA dataset is a large-scale visual question answering dataset with real images from the Visual Genome dataset and balanced question-answer pairs. Each training and validation image is also associated with scene graph annotations describing the classes and attributes of those objects in the scene, and their pairwise relations.

\paragraph{Text-VQA~\cite{singh2019towards}~(27k)} TextVQA is a dataset specifically designed to evaluate the ability of models to understand and answer questions about text embedded within images. Unlike traditional visual question answering (VQA) datasets that focus primarily on objects and scenes, TextVQA emphasizes the importance of reading and comprehending text in images.

\paragraph{OCR-VQA~\cite{mishra2019ocr}~(11K)} OCR-VQA (Optical Character Recognition Visual Question Answering) is a dataset specifically created to evaluate the ability of models to answer questions about images that contain text, with a strong emphasis on reading and understanding the text present in those images. This dataset is tailored to assess how well models can integrate OCR technology with visual question answering capabilities.

\paragraph{A-OK-VQA~\cite{schwenk2022okvqa}~(17K)} A crowdsourced dataset composed of a diverse set of about 25K questions requiring a broad base of commonsense and world knowledge to answer. In contrast to existing knowledge-based VQA datasets, the questions generally cannot be answered by simply querying a knowledge base, and instead require some form of commonsense reasoning about the scene depicted in the image.

\paragraph{ScienceQA~\cite{lu2022learn}~(13K)} 
ScienceQA is a dataset designed to evaluate models' abilities to understand and reason about science-related content presented in a multimodal format, including text, images, and diagrams. This dataset is particularly useful for assessing models' capabilities in understanding scientific concepts, interpreting visual information, and applying reasoning skills to answer questions accurately.

\paragraph{ST-VQA~\cite{biten2019scene}~(26K)} ST-VQA (Scene Text Visual Question Answering) is a dataset designed to evaluate the ability of models to understand and answer questions about images containing text in natural scenes. This dataset emphasizes the integration of text recognition and visual understanding, making it particularly challenging and relevant for applications that require interpreting text within images. 

\paragraph{ViQuAE~\cite{lerner2022viquae}~(1K)} ViQuAE is the first dataset for Knowledge-based Visual Question Answering about Named Entities.

\paragraph{Visual Storytelling~\cite{huang2016visual}~(5K)} It is the first dataset of sequential images with corresponding descriptions, which captures some of these subtle but important differences, and advance the task of visual storytelling. The data is in three tiers of language for
the same images: (1) Descriptions of imagesin-isolation (DII); (2) Descriptions of images-insequence (DIS); and (3) Stories for images-insequence (SIS).

\paragraph{Visual Dialog~\cite{das2017visual}~(50K)} Visual Dialog is a dataset and benchmark designed to evaluate the ability of models to hold a meaningful conversation about images. Unlike traditional visual question answering (VQA), where a single question is asked about an image, Visual Dialog involves a sequence of questions and answers, requiring the model to maintain context and continuity throughout the dialogue.

\paragraph{Multi30k~\cite{elliott2016multi30k}~(90K)} This dataset extends the Flickr30K~\cite{young2014image} dataset with i) German translations created by professional translators over a subset of the English descriptions, and ii) descriptions crowdsourced independently of the original English descriptions.

\paragraph{COCO-Caption CN~\cite{li2019coco}~(18K)} COCO-CN is a novel dataset enriching MS-COCO with manually written Chinese sentences and tags.

\paragraph{Flickr-8k-Caption CN~\cite{li2016adding}~(6K)} Flickr8k-CN is a bilingual extension of the popular Flickr8k set. The new multimedia dataset can be used to quantitatively assess the performance of Chinese captioning and English-Chinese machine translation.

\paragraph{Multimodal Chat~\cite{zheng2021mmchat}~(3K)} MMChat is a large-scale Chinese multi-modal dialogue corpus (32.4M raw dialogues and 120.84K filtered dialogues). Unlike previous corpora that are crowd-sourced or collected from fictitious movies, MMChat contains image-grounded dialogues collected from real conversations on social media, in which the sparsity issue is observed.

\paragraph{FM-IQA~\cite{gao2015you}~(165K)} Freestyle Multilingual Image Question Answering (FM-IQA) dataset contains over 150,000 images and 310,000 freestyle Chinese question-answer pairs and their English translations.

\paragraph{ChineseFoodNet~\cite{chen2017chinesefoodnet}~(1K)} ChineseFoodNet aims to automatically recognizing pictured Chinese dishes. The images of each food category consists of not only web recipe and menu pictures but photos taken from real dishes, recipe and menu as well. ChineseFoodNet contains over 180,000 food photos of 208 categories.

\paragraph{Evol-Intruct-GPT4-Turbo-143K~\cite{chen2024allava}~(143K)} They choose WizardLM-evol-instruct-V2~\cite{xu2023wizardlm} as the question set and regenerate the answers using GPT4-Turbo.

\paragraph{ShareGPT4V~\cite{chen2023sharegpt4v}~(100K)} ShareGPT4V originates from a curated 100K high-quality captions collected from advanced GPT4-Vision.

\paragraph{ALLaVA-Caption-LAION-4V~\cite{chen2024allava}~(506K)} The source images are from LAION dataset~\cite{schuhmann2022laion}. It asks GPT-4V to keep an eye on multiple aspects of an image and describe the image as detail as possible. The generated caption is expected to be rich, which is organized in certain logic by GPT-4V.

\paragraph{ALLaVA-Caption-VFLAN-4V~\cite{chen2024allava}~(203K)} The source images are from VFLAN dataset~\cite{dai2024instructblip}. It asks GPT-4V to keep an eye on multiple aspects of an image and describe the image as detail as possible. The generated caption is expected to be rich, which is organized in certain logic by GPT-4V.

\paragraph{LLaVA-Mix-665K~\cite{liu2023improved}~(665K)} LLaVA-Mix-665K is an instruction-following dataset mixed from 10 academically oriented datasets processed by LLaVA~\cite{liu2023improved}.

\paragraph{LVIS-Instruct4V~\cite{wang2023see}~(220K)} They use 110K images from LVIS~\cite{gupta2019lvis} and generate 220K high-quality visual instructions, which consist of 110K conversational data and 110K descriptional data.

\paragraph{ALLaVA-Instruct-LAION-4V~\cite{chen2024allava}~(506K)} They prompt GPT-4V with an image, and ask it to first generate a fine-grained caption then a VQA pair. By doing so, the whole data synthesis procedure including three stages: captioning, questioning and answering.

\paragraph{ALLaVA-Instruct-VFLAN-4V~\cite{chen2024allava}~(203K)} For Vision-FLAN dataset, the original answers have formatting issues or even incomplete as sentences; therefore, directly learning on such outputs may harm the fluency and coherence of the language model. They manually checked a few GPT-4V answered output and its quality is satisfied.

\paragraph{ShareGPTVideo-Caption~\cite{zhang2024direct}~(901K)} The dataset includes videos from three sources: WebVid~\cite{bain2021frozen} and VIDAL~\cite{zhu2023languagebind}, which are general domain videos from YouTube with 400k and 450k sampled videos respectively, and the ActivityNet~\cite{caba2015activitynet} dataset, which adds 50k videos focusing on human activities. Together, these three datasets provide a comprehensive collection of 900k videos. To meet the requirement that GPT-4V only accepts images as input, we preprocess the videos by uniformly extracting ten frames from each video. These frames are then concatenated into a sequence to serve as a proxy for the video. This sequence is input into GPT-4V to generate a coherent caption based on the frame sequence. The prompt follows guidelines covering temporal dynamics, world knowledge, object attributes, spatial relationships, aesthetic assessments, etc., with the aim of fully understanding the video contents.

\paragraph{ShareGPTVideo-QA~\cite{zhang2024direct}~(905K)} To generate video instruction-following data for supervised fine-tuning, they follow a methodology similar to that described in Video-ChatGPT~\cite{maaz2023video}, starting by randomly sampling 20K, 30K, and 30K captions from our dataset, specifically from ActivityNet, WebVid, and VIDAL, respectively. ChatGPT create three question-answer pairs for each detailed video caption, resulting in a total of 240k instruction data points for fine-tuning. This method ensures that the instructional data remains factually consistent with the content of the detailed captions.

\paragraph{FaceCaption~\cite{dai202415mmultimodalfacialimagetext}~(100K)} FaceCaption-15M comprises over 15 million pairs of facial images and their corresponding natural language descriptions of facial features, making it the largest facial image-caption dataset to date. We conducted a comprehensive analysis of image quality, text naturalness, text complexity, and text-image relevance to demonstrate the superiority of FaceCaption-15M.

\paragraph{ShareGPT4Video~\cite{chen2024sharegpt4video}~()} It contains 40K GPT4V annotated dense captions of videos with various lengths and sources, developed through carefully designed data filtering and annotating strategy.

\paragraph{M4-Instruct~\cite{liu2024llavanext}~()} M4-Instruct is a set of multi-image datasets that are collected from public datasets or generated by the GPT-4V API. It is constructed for training LMMs for their interleaved multi-image capbilities, \eg, LLaVA-NeXT-Interleave.

\paragraph{Cambrian~\cite{tong2024cambrian}~()} Cambrian-10M is a large-scale dataset designed for training Multimodal Large Language Models (MLLMs). It contains over 10 million visual instruction tuning data points, sourced from Visual Question Answering (VQA), visual conversations, and embodied visual interactions. From this, a curated subset called Cambrian-7M, with 7 million high-quality data points, was created to improve model training and performance. The dataset includes extended responses generated by GPT-4v and creative data from GPT-4o, addressing issues like short VQA outputs and limited science-related data. By introducing system prompts, Cambrian-7M enhances the model’s creativity and mitigates the "Answer Machine" phenomenon, encouraging more interactive responses.

\paragraph{DenseFusion~\cite{li2024densefusion}~()} DenseFusion-1M dataset is collected for highly informative image descriptions with various visual details, including rich OCR information, accurate object and position recognition, and external knowledge, \etc.

\paragraph{MiraData~\cite{ju2024miradata}~()} They curate MiraData from diverse, manually selected sources and meticulously process the data to obtain semantically consistent clips. GPT-4V is employed to annotate structured captions, providing detailed descriptions from four different perspectives along with a summarized dense caption
